# Supplementary material for: Exploring Image Representation with Decoupled Classical Visual Descriptors
Source: arXiv:2510.14536 source file (2025-10-16)
Supplement: Supplementary file 1 [file surveytable.tex]

% \begin{table*} [t]
% \centering
% \caption{Survey results for different models on image colour editing task with three attributes. }
% \begin{tabularx}{\linewidth}{|c|>{\centering\arraybackslash}X|>{\centering\arraybackslash}X|>{\centering\arraybackslash}X|>{\centering\arraybackslash}X|}
% \hline
% \multirow{2}{*}{\textbf{Attributes}} & \multicolumn{4}{c|}{\textbf{Model}} \\ \cline{2-5} 
%                                   &\textbf{Controlnet} & \textbf{T2I-Adapter} & \textbf{ControlNet ++} & 
%                                   \textbf{Ours}
%                                   \\ 
%                                   \hline
% Naturalness &&&&\\ \hline
% Accuracy &&&&\\ \hline
% Consistency &&&&\\ \hline
                                  
% \end{tabularx}
% \label{tab: survey table}
% \end{table*}

\begin{table*} [t]
\centering
\caption{Survey results for different models on the image colour editing task with attributes. }
\vspace{1.5mm}
\begin{tabular}{c | c c c}
\toprule
                            Models      &\textbf{Naturalness} & \textbf{Accuracy} &
                                  \textbf{Consistency}
                                  \\ 
                                  \midrule
ControlNet~\cite{zhang2023adding} w/ prompt&2.02&2.89&2.06\\ 
T2I Adapter~\cite{mou2024t2i} w/ prompt&2.72&3.10&2.13\\ 
ControlNet++~\cite{li2025controlnet} w/ prompt&2.32&3.41&2.33\\ 
Ours           &\textbf{4.13}&\textbf{4.16}&\textbf{4.25}\\ 
\bottomrule
\end{tabular}
\label{tab:survey_table}
\end{table*}

% \begin{table*}[t]
% \centering
% \caption{Survey results for different models on the image colour editing task with attributes.}
% \label{tab:survey_table}
% \renewcommand{\arraystretch}{1.2} % Adjust row height for better readability
% \begin{tabular}{|l|c|c|c|}
% \hline
% \textbf{Models} & \textbf{Naturalness} & \textbf{Accuracy} & \textbf{Consistency} \\ 
% \hline
% ControlNet~\cite{zhang2023adding} w/ prompt & 2.02 & 2.89 & 2.06 \\ 
% \hline
% T2I Adapter~\cite{mou2024t2i} w/ prompt & 2.72 & 3.10 & 2.13 \\ 
% \hline
% ControlNet++~\cite{li2025controlnet} w/ prompt & 2.32 & 3.41 & 2.33 \\ 
% \hline
% Ours & \textbf{4.13} & \textbf{4.16} & \textbf{4.25} \\ 
% \hline   
% \end{tabular}
% \end{table*}
