# Supplementary material for: Exploring Image Representation with Decoupled Classical Visual Descriptors
Source: arXiv:2510.14536 source file (2025-10-16)
Supplement: Supplementary file 2 [file LPIPS_abalation.tex]

\begin{table*} [t]
\centering
\caption{Comparative performance with and without LPIPS and MSE losses in Linear Probing and Finetuning over training steps}
    \vspace{1.5mm}
\begin{tabular}{c| c c c| c c c}
\toprule
\multirow{2}{*}{\textbf{\#steps}} & \multicolumn{3}{c|}{\textbf{Linear Probing}} & \multicolumn{3}{c}{\textbf{Fine-tuning}} \\ \cline{2-7} 
                                  & \textbf{ours} & \textbf{w/o LPIPS} & 
                                  \textbf{w/o MSE} & \textbf{ours} & \textbf{w/o LPIPS} & 
                                  \textbf{w/o MSE}
                                  \\ 
                                  \midrule

100k  & 22.5 & 22.7 \p{0.2} & 17.7 \m{4.8} & 70.9 & 71.0 \p{0.1} &70.0 \m{0.9}\\
200k  & 42.2 & 42.6 \p{0.4} & 37.1 \m{5.1} & 75.7 & 75.6 \m{0.1}& 74.5 \m{1.2}\\ 
400k  & 55.9 & 56.0 \p{0.1}& 50.3 \m{5.6}& 78.8 & 78.8 \e{0.0}& 78.1 \m{0.7}\\ 
800k  & 64.7 & 64.6 \m{0.1}& 60.1\m{4.6} & 81.1 & 80.9 \m{0.2}& 80.7 \m{0.4}\\ 
1600k & 69.6 & 69.2 \m{0.4}& 64.2 \m{5.4}& 82.7 & 82.3 \m{0.4} & 82.1 \m{0.6}\\ 
3200k & 72.6 & 71.9 \m{0.7}& 65.6 \m{7.0}& 83.3 & 83.0 \m{0.3}& 82.6 \m{0.7}\\ 
6400k & 74.0 & 73.0 \m{1.0}& 66.5 \m{7.5}& 83.5 & 83.1\m{0.4}& 82.6\m{0.9}\\ \bottomrule
\end{tabular}
\label{tab: LPIPS Abalation}
\end{table*}
