# Supplementary material for: Exploring Image Representation with Decoupled Classical Visual Descriptors
Source: arXiv:2510.14536 source file (2025-10-16)
Supplement: Supplementary file 3 [file Loss_Reconstruction_Ablation.tex]

\begin{table} [t]
\centering
\caption{Quantitative results of the pre-training image restoration task. The results are presented in PSNR/SSIM. }
\vspace{1.5mm}
\begin{tabular}{c c c}
\toprule
                                   \textbf{w/o LPIPS} & \textbf{w/o MSE} & \textbf{Full}
                                  \\ 
                                  \midrule
29.71/ 0.6012 & 30.72/ 0.6133 & \textbf{31.42/ 0.8409} \\
\bottomrule
\end{tabular}
\label{tab: Loss Reconstruction Abalation}
\end{table}
