# Supplementary material for: Exploring Image Representation with Decoupled Classical Visual Descriptors
Source: arXiv:2510.14536 source file (2025-10-16)
Supplement: Supplementary file 4 [file decoder_blocks.tex]

\begin{table}[t]
\centering
\caption{Comparative performance with different number of decoder blocks in Linear Probing and Finetuning}
    \vspace{2mm}
\begin{tabular}{c c c c c c c}
% \hline
\toprule
{Block} &  1 &  2 & 4 & 8 & 12 & 24 \\ \midrule

{Linear Probing}  &60.2&  68.8&  72.5 &  \textbf{74.0} & 73.6 & 73.4\\ 
{Fine-tuning}  &82.9 & 83.4 &  83.4 & \textbf{83.5}& 83.4&83.4
 \\ \bottomrule

\end{tabular}
\label{supptab: decoder blocks}
\end{table}
