# Supplementary material for: Exploring Image Representation with Decoupled Classical Visual Descriptors
Source: arXiv:2510.14536 source file (2025-10-16)
Supplement: Supplementary file 5 [file descriptor_abalation.tex]

\begin{table} [t]
\centering
\caption{Comparative Performance with and without descriptor loss in Linear Probing and Fine-tuning Over Training Steps. Early stopping may intervene to prevent overfitting. Descriptor loss is notated as $L_d$.}
\vspace{1.5mm}
\begin{tabular}{c| c c| c c}
\toprule
\multirow{2}{*}{\textbf{\#steps}} & \multicolumn{2}{c|}{\textbf{Linear Probing}} & \multicolumn{2}{c}{\textbf{Fine-tuning}} \\ \cline{2-5} 
                                  & \textbf{ours} & \textbf{w/o $L_d$} & \textbf{ours} & \textbf{w/o $L_d$}
                                  \\ 
                                  \midrule

100k  & 22.5 & 17.7\m{4.8}  & 70.9 & 68.9\m{2.0} \\
200k  & 42.2 & 34.8\m{7.4}  & 75.7 & 72.7\m{3.0}\\ 
400k  & 55.9 & 48.3\m{7.6}& 78.8 & 76.3\m{2.5}\\
800k  & 64.7 & 58.5\m{6.2}&  81.1 & 79.3\m{1.8}\\ 
1600k & 69.6 & 63.6\m{6.0}& 82.7 & 81.1\m{1.6} \\ 
3200k & 72.6 & 65.8\m{6.8}&  83.3 & 82.2\m{1.1}\\ 
6400k & 74.0 & 66.8\m{8.0}& 83.5 & 82.8\m{0.7}\\ \bottomrule
\end{tabular}
\label{tab: descriptor Abalation}
\end{table}
