# Supplementary material for: Exploring Image Representation with Decoupled Classical Visual Descriptors
Source: arXiv:2510.14536 source file (2025-10-16)
Supplement: Supplementary file 6 [file implementation_details.tex]

\begin{table*}[ht]
    \centering
        \caption{Implementation hyper-parameter details.}
            \vspace{2mm}
    \begin{tabularx}{1\textwidth}{ >{\raggedright\arraybackslash}X |>{\centering\arraybackslash}X >{\centering\arraybackslash}X >{\centering\arraybackslash}X }
    \toprule
    Config & Pre-training & Fine-tuning & Linear Probing\\
    \midrule
        optimizer &  AdamW & AdamW & AdamW\\
         learning rate &1.5e-4&1.0e-3&1.0e-1\\
         weight decay        &1e-5&1e-5&0\\
         $\beta_1$ &0.95&0.95&0.9\\
         $\beta_2$&0.999&0.999&0.999\\
         $\epsilon$  &1e-8&1e-8&1e-8\\
         batch size&128&128&256\\
         learning rate scheduler&cosine decay&cosine decay&cosine decay\\
         warmup steps&1000&1000&500\\
         image size&224&224&224\\
         data normalisation&\cmark&\cmark&\xmark\\
         image mean&(0.485, 0.456, 0.406)&(0.485, 0.456, 0.406)&---\\
      standard deviation&(0.229, 0.224, 0.225)&(0.229, 0.224, 0.225)&---\\
      \bottomrule
        
   \end{tabularx}

    \label{tab:implementation_detail}
\end{table*}
