# Supplementary material for: Exploring Image Representation with Decoupled Classical Visual Descriptors
Source: arXiv:2510.14536 source file (2025-10-16)
Supplement: Supplementary file 7 [file latent_length.tex]

\begin{table}[t]
\centering
\caption{Comparative performance with different latent vector length in Linear Probing and Finetuning}
    \vspace{1.5mm}
\begin{tabular}{c c c c c c}
% \hline
\hline
{Length} &  128 &  256 & 512 & 768 & 1024 \\ \hline

{Linear Probing}  &61.5 & 68.9 &  73.5 &  74.0 & \textbf{74.6}  \\ 
{Fine-tuning}  &75.1 & 80.1  &  83.3 & 83.5 & \textbf{83.6}
 \\ \hline  
\end{tabular}
\label{supptab: vector length}
\end{table}
